# Supplementary material for: BOAssembler: a Bayesian Optimization Framework to Improve RNA-Seq Assembly Performance
Source: arXiv:1902.05235 source file (2019-02-14)
Supplement: Supplementary file 1 [file appendix.tex]

\subsection{BO improvements}

\subsubsection{Improve performance against BO's randomness}
BO's randomness come from the acquisition selection with randomness, which lead to undesired local optimum parameters lead to staled performance. To avoid BO getting stuck, one practical suggestion to conduct multiple BO runs.

\subsubsection{Avoid BO Overfitting by cross-validation}
BO is tuning parameters $\theta$ on small dataset, and test the performance on large dataset, which draws concern on overfitting. BO overfitting means parameter $\theta$ is over-optimized for the small dataset, while the performance on large dataset degrades.

We use additional validation dataset and early stopping to avoid BO overfitting. We take two small datasetof reads, $D_{train}$ is for training and $D_{val}$ for validation. $f(.)$ is optimized solely on $D_{train}$ to get $\theta_t$, while for each iteration the $f(D_{val}, \theta_t)$ is evaluated. After all iterations, the best parameter evaluated on $D_{val}$ is returned. Use the cross-validation on BO, we avoid overfitting parameter to training dataset.\textbf{Some experiment to support?}
